# Supplementary material for: Phase-space iterative solvers
Source: arXiv:2309.14031 source file (2024-11-24)
Supplement: Supplementary file 1 [file Generalizing.tex]

\paragraph{Friedrichs angle for more elements in 1D}

In this case, we will consider the same setting of our reference problem, but with more than one discretization element.
Let us assume, to start, the simplest case, which is $N_e=2$ in 1D, with $L_{e1}=L_{e2}$, so that the two elements have the same length. The Young Modulus Y associated to each discretization element is always the same. Consider the definition of Friedrichs angle in eq. (\ref{friedrichsangle}) and the scalar product as defined in eq. (\ref{eq:scalarprod}). We have that the global phase space vector $z$ has four components, which we can rewrite as:
\begin{align}
{z} &= \begin{bmatrix} \varepsilon_{1} \quad \sigma_{1}  \quad \varepsilon_{2} \quad \sigma_{2}\end{bmatrix}^\top
\end{align}

and we can define the "subspaces" associated respectively to the phisically-admissible and materially-admissible set as:

\[
\mathcal{M}_1:=\left\{\sigma_1,\sigma_2=F/A=\widetilde{\sigma}, \forall \varepsilon_1,\varepsilon_2\right\}
\]
\[
\mathcal{M}_2:=\left\{\sigma_1=Y\varepsilon_1, \forall \varepsilon_1; \sigma_2=Y\varepsilon_2, \forall \varepsilon_2\right\}
\]

notice that also in this case, $\mathcal{M}_1$ does not represent a subspace. However, one can consider a shifted version which contains the zero vector, without affecting the value of the angle). We will rewrite:
\[
\mathcal{M}_1:=\left\{\sigma_1,\sigma_2=0, \forall \varepsilon_1,\varepsilon_2\right\}
\]
which actually represents a subspace.

Also in this case we can see that:
$M = \mathcal{M}_1 \cap \mathcal{M}_2$=$\left\{{0} \right\}$

hence:
\[
M^\perp=\left\{v: v \neq {0} \right\}
\]

We now need to define two vectors $ \in \mathbb{R}^4$, which are x:=$\left\{x \in \mathcal{M}_1: \left\| x \right\|=1\right\}$, and y:=$\left\{y \in \mathcal{M}_2: \left\| y \right\|=1\right\}$.
One needs to choose these vectors so that the $sup$ of the scalar product is maximized in eq. (\ref{friedrichsangle}). This requires to solve a constraint optimization problem. We will consider the case where the force applied is positive, so that $\varepsilon, \sigma >0$. We proceed using Lagrange Multipliers, under the hypothesis $x,y$ positive vectors. Obviously, the $sup$ is attained at the frontiers of the two unitary balls. So, we can rewrite the constraints associated to the subspaces $\mathcal{M}_1$, and $\mathcal{M}_2$, considering the squared norm inside the definition of unitary ball in eq.(\ref{ball}). Clearly, requiring the norm or the squared norm to be equal to one is equivalent.\\
We have that ${w_e}=L_{e}A$, assuming the cross section area $A$ equal for all elements.\\
For the subspace $\mathcal{M}_1$, we want the unitary ball constraint to be enforced via Lagrange Multipliers:
\begin{equation}
\frac{w_1}{2} \left[ C \varepsilon_1^{2} \right]+\frac{w_2}{2} \left[ C \varepsilon_2^{2}\right]=1
\end{equation}
which leads to the function:
\begin{equation}
g1(\varepsilon_1,\varepsilon_2)  = \frac{w_1}{2} \left[ C \varepsilon_1^{2} \right]+\frac{w_2}{2} \left[ C \varepsilon_2^{2}\right]-1=0
\end{equation}
For $\mathcal{M}_2$ instead, we have that:
\begin{equation}
\frac{w_1}{2} \left[ C \varepsilon_1^{2}+C^{-1}\sigma_1^{2} \right]+\frac{w_2}{2} \left[ C \varepsilon_2^{2}+C^{-1}\sigma_2^{2}\right]=1
\end{equation}

which boils down to:

\begin{equation}
\frac{w_1}{2} \left[ C \varepsilon_1^{2}+C^{-1}\varepsilon_1^{2}Y^{2} \right]+\frac{w_2}{2} \left[ C \varepsilon_2^{2}+C^{-1}\varepsilon_2^{2}Y^{2}\right]=1
\end{equation}

and can be rewritten as a function:

\begin{equation}
g2(\varepsilon_1,\varepsilon_2) =\frac{w_1}{2} \left[ C \varepsilon_1^{2}+C^{-1}\varepsilon_1^{2}Y^{2} \right]+\frac{w_2}{2} \left[ C \varepsilon_2^{2}+C^{-1}\varepsilon_2^{2}Y^{2}\right]-1=0
\end{equation}

In this way, we have that the two vectors $x,y$ are defined as:

$x$:=
$
\begin{pmatrix}
\varepsilon_{1} \quad
\sigma_{1} \quad
\varepsilon_{2} \quad
\sigma_{2}
\end{pmatrix}^\top
=\begin{pmatrix}
\varepsilon_{1,x} \quad
0 \quad
\varepsilon_{2,x} \quad
0
\end{pmatrix}^\top\\
$
$y$:=
$
\begin{pmatrix}
\varepsilon_{1} \quad
\sigma_{1} \quad
\varepsilon_{2} \quad
\sigma_{2}
\end{pmatrix}^\top
=\begin{pmatrix}
\varepsilon_{1,y} \quad
Y\varepsilon_{1,y}  \quad
\varepsilon_{2,y} \quad
Y\varepsilon_{2,y}
\end{pmatrix}^\top
$.\\
\\
Introducing the Lagrange Multipliers $\lambda_{1}$ and $\lambda_{2}$, where the first constraint $g1$ is associated to $x$ and where the second constraint $g2$ is associated to $y$, and using eq.(\ref{friedrichsangle}) and (\ref{eq:scalarprod}), the problem of finding the maximum scalar product under the two mentioned constraints, becomes equivalent to finding the maximum of the following function of $\varepsilon_{1,x}, \varepsilon_{2,x}, \varepsilon_{1,y}, \varepsilon_{2,y}, \lambda_{1}, \lambda_{2}$:

\begin{equation}
f(\varepsilon_{1,x}, \varepsilon_{2,x}, \varepsilon_{1,y}, \varepsilon_{2,y}, \lambda_{1}, \lambda_{2})=\frac{w_1}{2} [ \varepsilon_{1,x} C \varepsilon_{1,y}]+\frac{w_2}{2} [ \varepsilon_{2,x} C \varepsilon_{2,y}]-\lambda_{1}g1(\varepsilon_{1,x},\varepsilon_{2,x})-\lambda_{2}g2(\varepsilon_{1,y},\varepsilon_{2,y})
\end{equation}

explicitly written as:

\begin{align*}
f(\varepsilon_{1,x}, \varepsilon_{2,x}, \varepsilon_{1,y}, \varepsilon_{2,y}, \lambda_{1}, \lambda_{2})=
\frac{w_1}{2} [ \varepsilon_{1,x} C \varepsilon_{1,y}]+\frac{w_2}{2} [ \varepsilon_{2,x} C \varepsilon_{2,y}]-\lambda_{1}(\frac{w_1}{2} \left[ C \varepsilon_{1,x}^{2} \right]+\frac{w_2}{2} \left[ C \varepsilon_{2,x}^{2}\right]-1)\\-\lambda_{2}(\frac{w_1}{2} \left[ C \varepsilon_{1,y}^{2}+C^{-1}\varepsilon_{1,y}^{2}Y^{2} \right]+\frac{w_2}{2} \left[ C \varepsilon_{2,y}^{2}+C^{-1}\varepsilon_{2,y}^{2}Y^{2}\right]-1)
\end{align*}

We can take partial derivatives so that:

\begin{equation}
\left\{
\begin{aligned}
    \frac{\partial f}{\partial \varepsilon_{1,x}} &= 0 \\
    \frac{\partial f}{\partial \varepsilon_{2,x}} &= 0 \\
    \frac{\partial f}{\partial \varepsilon_{1,y}} &= 0 \\
    \frac{\partial f}{\partial \varepsilon_{2,y}} &= 0 \\
    \frac{\partial f}{\partial \lambda_{1}} &= 0 \\
    \frac{\partial f}{\partial \lambda_{2}} &= 0
\end{aligned}
\right.
\end{equation}

leading to the system of equations:

\begin{equation}
\left\{
\begin{aligned}
    &\frac{w_1}{2} ( C \varepsilon_{1,y})= \lambda_{1}({w_1} C \varepsilon_{1,x}) \\
    &\frac{w_2}{2} ( C \varepsilon_{2,y})= \lambda_{1}({w_2} C \varepsilon_{2,x}) \\
    &\frac{w_1}{2} ( C \varepsilon_{1,x}) = \lambda_{2}{w_1}(\varepsilon_{1,y}+C^{-1}\varepsilon_{1,y}Y^{2}) \\
    &\frac{w_2}{2} ( C \varepsilon_{2,x}) = \lambda_{2}{w_2}(\varepsilon_{2,y}+C^{-1}\varepsilon_{2,y}Y^{2}) \\
    &\frac{w_1}{2} \left( C \varepsilon_{1,x}^{2} \right)+\frac{w_2}{2} \left( C \varepsilon_{2,x}^{2}\right) = 1 \\
    &\frac{w_1}{2} \left( C \varepsilon_{1,y}^{2}+C^{-1}\varepsilon_{1,y}^{2}Y^{2} \right)+\frac{w_2}{2} \left( C \varepsilon_{2,y}^{2}+C^{-1}\varepsilon_{2,y}^{2}Y^{2}\right)=1
\end{aligned}
\right.
\label{fullsystem}
\end{equation}

which can be further simplified into:

\begin{equation}
\left\{
\begin{aligned}
    & \varepsilon_{1,y}= 2\lambda_{1} \varepsilon_{1,x} \\
    &\varepsilon_{2,y}= 2\lambda_{1}\varepsilon_{2,x} \\
    &C \varepsilon_{1,x} = 2\lambda_{2}(\varepsilon_{1,y}+C^{-1}\varepsilon_{1,y}Y^{2}) \\
    & C \varepsilon_{2,x} =2\lambda_{2}(\varepsilon_{2,y}+C^{-1}\varepsilon_{2,y}Y^{2}) \\
    &\frac{w_1}{2} \left( C \varepsilon_{1,x}^{2} \right)+\frac{w_2}{2} \left( C \varepsilon_{2,x}^{2}\right) = 1 \\
    &\frac{w_1}{2} \left( C \varepsilon_{1,y}^{2}+C^{-1}\varepsilon_{1,y}^{2}Y^{2} \right)+\frac{w_2}{2} \left( C \varepsilon_{2,y}^{2}+C^{-1}\varepsilon_{2,y}^{2}Y^{2}\right)=1
\end{aligned}
\right.
\end{equation}

At this stage we can introduce the hypothesis of equal lengths of the two elements, as mentioned before, so that ${w_1}={w_2}={w}$. This allows to simplify the system with $\varepsilon_{1,x}=\varepsilon_{2,x}=\varepsilon_{x}$, and $\varepsilon_{1,y}=\varepsilon_{2,y}=\varepsilon_{y}$.
From the last two equations, for a suitable choice of $\lambda_{1}$ and $\lambda_{2}$, we have that a solution is given by: 

\begin{equation}
{w} \left( C \varepsilon_{x}^{2} \right) = 1
\end{equation}

so that 

\begin{equation}
\varepsilon_{x} = (\frac{1}{wC})^{\frac{1}{2}}
\end{equation}

and also:

\begin{equation}
{w} \left( C \varepsilon_{y}^{2}+C^{-1}\varepsilon_{y}^{2}Y^{2} \right)=1
\end{equation}

in order to obtain:

\begin{equation}
\varepsilon_{y}={(\frac{C}{wC^{2}+wY^2})}^{\frac{1}{2}}
\end{equation}

ending up with:

$x$:$
=\begin{pmatrix}
\varepsilon_{x} \quad
0 \quad
\varepsilon_{x} \quad
0
\end{pmatrix}^\top\\
$
$y$:
=$\begin{pmatrix}
\varepsilon_{y} \quad
Y\varepsilon_{y}  \quad
\varepsilon_{y} \quad
Y\varepsilon_{y}
\end{pmatrix}^\top$

now the cosine of the Friedrichs angle could be computed as from the definition:

\[
 \left| \langle x, y \rangle \right|= \frac{w_1}{2} [ \varepsilon_{1,x} C \varepsilon_{1,y} + \sigma_{1,x} C^{-1} \sigma_{1,y}]+\frac{w_2}{2} [ \varepsilon_{2,x} C \varepsilon_{2,y} + \sigma_{2,x} C^{-1} \sigma_{2,y}]
\]

which in this case reduces to:

\[
 \left| \langle x, y \rangle \right|= {w} [ \varepsilon_{x} C \varepsilon_{y} ]=C {(\frac{1}{(C^2+Y^2)})}^{\frac{1}{2}}={(\frac{1}{(1+\alpha^2)})}^{\frac{1}{2}}
\]

now exploiting eq. (\ref{eq:convrate}) the convergence rate is defined by the square of the previous quantity, namely:

\[
\frac{1}{1+\alpha^2}
\]

which coincides with the result derived for one element. In the general case where $Ne$>2, and assuming ${w_1}={w_2}=...={w_e}={w}$, we can also always assume that $\varepsilon_{1,x}=\varepsilon_{2,x}=...=\varepsilon_{e,x}=\varepsilon_{x}$, and $\varepsilon_{1,y}=\varepsilon_{2,y}=...=\varepsilon_{e,y}=\varepsilon_{y}$. The system of equations (\ref{fullsystem}) will have $2Ne+2$ equations, where the last two are associated to the Lagrange Multipliers of the unitary ball constraints for subspaces $\mathcal{M}_1$ and $\mathcal{M}_2$. The solutions for $\varepsilon_{x}$ and $\varepsilon_{y}$ would be same as the case for 2 elements, accounting for a prefactor $1/Ne$. However, in the definition of scalar product, the equation can be rewritten as a num over $Ne$ of a constant quantity, hence the prefactor $1/Ne$ is eliminated by this sum. This proofs that the Friedrichs angle is preserved in the global pahse space independently of the number of discretzation elements, and that the convergence rate is not affected by that, under the assumptions mentioned above.

\paragraph{Friedrichs angle for more elements with different volumes in 1D}

In the previous section, the hypothesis of elements with equal volume has been added. In the following, we would like to relax this assumption, considering elements with different lengths but same cross section area. The case where $Ne=2$ will we considered, in order to show that the Friedrichs angle is preserved also under such condition. Without any assumption on the volume of the elements, the two vectors $x,y$ which define the Friedrichs angle, are:

$x$:=$
\begin{pmatrix}
\varepsilon_{1} \quad
\sigma_{1} \quad
\varepsilon_{2} \quad
\sigma_{2}
\end{pmatrix}
=\begin{pmatrix}
\varepsilon_{1,x} \quad
0 \quad
\varepsilon_{2,x} \quad
0
\end{pmatrix}^\top\\
$
$y$:=$
\begin{pmatrix}
\varepsilon_{1} \quad
\sigma_{1} \quad
\varepsilon_{2} \quad
\sigma_{2}
\end{pmatrix}^\top
=\begin{pmatrix}
\varepsilon_{1,y} \quad
Y\varepsilon_{1,y}  \quad
\varepsilon_{2,y} \quad
Y\varepsilon_{2,y}
\end{pmatrix}^\top
$.\\
\\
The solution is given by the set of equations:

\begin{equation}
\left\{
\begin{aligned}
    & \varepsilon_{1,y}= 2\lambda_{1} \varepsilon_{1,x} \\
    &\varepsilon_{2,y}= 2\lambda_{1}\varepsilon_{2,x} \\
    &C \varepsilon_{1,x} = 2\lambda_{2}(\varepsilon_{1,y}+C^{-1}\varepsilon_{1,y}Y^{2}) \\
    & C \varepsilon_{2,x} =2\lambda_{2}(\varepsilon_{2,y}+C^{-1}\varepsilon_{2,y}Y^{2}) \\
    &\frac{w_1}{2} \left( C \varepsilon_{1,x}^{2} \right)+\frac{w_2}{2} \left( C \varepsilon_{2,x}^{2}\right) = 1 \\
    &\frac{w_1}{2} \left( C \varepsilon_{1,y}^{2}+C^{-1}\varepsilon_{1,y}^{2}Y^{2} \right)+\frac{w_2}{2} \left( C \varepsilon_{2,y}^{2}+C^{-1}\varepsilon_{2,y}^{2}Y^{2}\right)=1
\end{aligned}
\right.
\end{equation}

in the general setting where no assumptions are given on the volumes, we can assume that $\varepsilon_{1,x}=M\varepsilon_{2,x}$, and $\varepsilon_{1,y}=M\varepsilon_{2,y}$ for a generic positive scaling parameter $M$. From the equations follows:

\begin{equation}
\varepsilon_{1,x} = M{(\frac{2}{(w_1M^2+w_2)C})}^{\frac{1}{2}}
\end{equation}

\begin{equation}
\varepsilon_{2,x} = {(\frac{2}{(w_1M^2+w_2)C})}^{\frac{1}{2}}
\end{equation}

\begin{equation}
\varepsilon_{1,y}=M{(\frac{2C}{(w_1M^2+w_2)(C^{2}+Y^2)})}^{\frac{1}{2}}
\end{equation}

\begin{equation}
\varepsilon_{2,y}={(\frac{2C}{(w_1M^2+w_2)(C^{2}+Y^2)})}    ^{\frac{1}{2}}
\end{equation}

now the cosine of the Friedrichs angle is:

\[
 \left| \langle x, y \rangle \right|= \frac{w_1}{2} [ \varepsilon_{1,x} C \varepsilon_{1,y} + \sigma_{1,x} C^{-1} \sigma_{1,y}]+\frac{w_2}{2} [ \varepsilon_{2,x} C \varepsilon_{2,y} + \sigma_{2,x} C^{-1} \sigma_{2,y}]
\]

simplified into:

\[
 \left| \langle x, y \rangle \right|= \frac{w_1}{2} [ \varepsilon_{1,x} C \varepsilon_{1,y}] +\frac{w_2}{2} [ \varepsilon_{2,x} C \varepsilon_{2,y} ]
\]

and by explicit computation:

\[
 \left| \langle x, y \rangle \right|= {w_1} [  M^2{(\frac{C^2}{(w_1M^2+w_2)^2(C^{2}+Y^2)})}^{\frac{1}{2}}] +{w_2} [ {(\frac{C^2}{(w_1M^2+w_2)^2(C^{2}+Y^2)})}^{\frac{1}{2}} ]={(
\frac{1}{1+\alpha^2})}^{\frac{1}{2}}
\]

and now exploiting eq. (\ref{eq:convrate}) we have that the convergence rate is defined by the square of the previous quantity, namely:

\[
\frac{1}{1+\alpha^2}
\]

It is worth noticing how the value of $M$ does not actually affect the Friedrichs angle.

In conclusion, the computations of this appendix show that the convergence properties of the method, in this specific example, are coherent with theoretical predictions, and are preserved independently of the number of discretization elements and of their volumes. Clearly, this example has a well known analytical solution, so it has been used as test case to analyze some properties of this iterative method in an abstract framework.
